# Supplementary material for: Inv-Adapter: ID Customization Generation via Image Inversion and Lightweight Adapter
Source: arXiv:2406.02881 source file (2024-06-06)
Supplement: Supplementary file 1 [file 06supp.tex]

\subsection{Broader Impact} \label{supp-1}
We propose Inv-Adapter, a lightweight approach to ID customisation generation. It requires only the base text-to-image model without additional cue image encoders to achieve high quality ID generation. Our approach achieves minimal model parameters and trainable parameters while achieving very competitive results.

\myparagraph{Positive impact:}
\begin{itemize}
    \item \textbf{Facilitating ID generation tasks}. We provide a novel solution to the ID customisation task by achieving high quality ID generation through image inversion. It only needs to be implemented by the text-to-image model itself without the need of additional image encoders.
    \item \textbf{Advancements in AIGC Research}. Our approach provides solutions to other AIGC tasks, such as anthing retention, out-paingting tasks, and can facilitate exploration of the AIGC field.
    \item \textbf{Facilitates end-side deployment.} Our approach does not rely on additional image encoders and helps in end-side deployment of AIGC applications.
\end{itemize}

\myparagraph{Negative impact:}
\begin{itemize}
\item \textbf{Risks of Portrait Rights}. ID preservation could trigger the rise of face-swapping apps, posing a risk.
\item \textbf{Risk of False News.} When ID fidelity is sufficient it may trigger the spread of more disinformation.
\end{itemize}
\subsection{Details}
%%%%%%%%%%%
\myparagraph{Text Prompts.}
The proposed method constructs 42 text prompt templates to evaluate the loyalty of all methods. We follow the setting of Photomaker~\cite{li2023photomaker} and all prompts are shown below, where ``\{\}'' can be replaced by ``man/woman''.
\begin{lstlisting}
prompt_templete= [
  "a photo of a {}",
  "a {} wearing a spacesuit",
  "a {} wearing a red sweater",
  "a {} wearing a white shirt",
  "a {} wearing a red hat",
  "a {} wearing a blue hoodie",
  "a {} wearing headphones",
  "a {} with red hair",
  "a {} wearing headphones with red hair",
  "a {} wearing a Christmas hat",
  "a {} wearing sunglasses",
  "a {} wearing sunglasses and necklace",
  "a {} wearing a blue cap",
  "a {} wearing a doctoral cap",
  "a {} with white hair, wearing glasses",
  "a {} in a helmet and vest riding a motorcycle",
  "a {} holding a bottle of red wine",
  "a {} driving a bus in the desert",
  "a {} playing basketball",
  "a {} playing the violin",
  "a {} piloting a spaceship",
  "a {} riding a horse",
  "a {} coding in front of a computer",
  "a {} playing the guitar",
  "a {} laughing on the lawn",
  "a {} frowning at the camera",
  "a {} happily smiling, looking at the camera",
 " a {} crying disappointedly, with tears flowing",
  "a {} wearing sunglasses",
  "a {} playing the guitar in the view of left side",
 " a {} holding a bottle of red wine, upper body",
  "a {} wearing sunglasses and necklace, close-up,
        in the view of right side",
  "a {} riding a horse, in the view of the top",
  "a {} wearing a doctoral cap, upper body, with the 
       left side of the face facing the camera",
  "a {} crying disappointedly, with tears flowing, 
       with left side of the face facing the camera",
  "a {} sitting in front of the camera, with a 
       beautiful purple sunset at the beach in the background",
  "a {} swimming in the pool",
  "a {} climbing a mountain",
  "a {} skiing on the snowy mountain",
  "a {} in the snow",
  "a {} in space wearing a spacesuit",
  "a {} wearing a glasses, reading a book"
  ]
  \end{lstlisting}

\subsection{Supplementary Results} \label{supp}

\myparagraph{Inversion Image Quality.}
We indicate through the results of a large number of inversion experiments that for simple face images, the results obtained by DDIM inversion are of high quality. In general, almost no information is lost. While, for complex original images, the detail information is usually lost. 
\begin{wraptable}{r}{0.6\textwidth}
\centering
\vspace{-0.03cm}
\scriptsize
\setlength{\abovecaptionskip}{0cm}
\setlength{\belowcaptionskip}{-0.01cm}
\caption{L$_1$ loss obtained by DDIM inversion for the three datasets.}
\begin{tabular*}{0.99\linewidth} {@{\extracolsep{\fill}}c|ccc}
\hline
Datasets                 & Trainging dataset &sample-1K dataset& Celebrity dataset\\ \hline
L$_1$ loss &0.0566  &0.0340 & 0.0437 \\ \hline
\end{tabular*}\label{tabe1}
\vspace{-0.3cm}
\end{wraptable}
Table~\ref{tabe1} shows the L$_1$ error obtained by DDIM inversion for the face images of training set, inference set. It can be found that DDIM inversion high quality recovered original images. Therefore, DDIM inversion can be used for face feature extraction in the proposed method without losing detail information.

\begin{figure}[h!]
    \centering\setlength{\abovecaptionskip}{0.1cm}
    \includegraphics[width=0.99\linewidth]{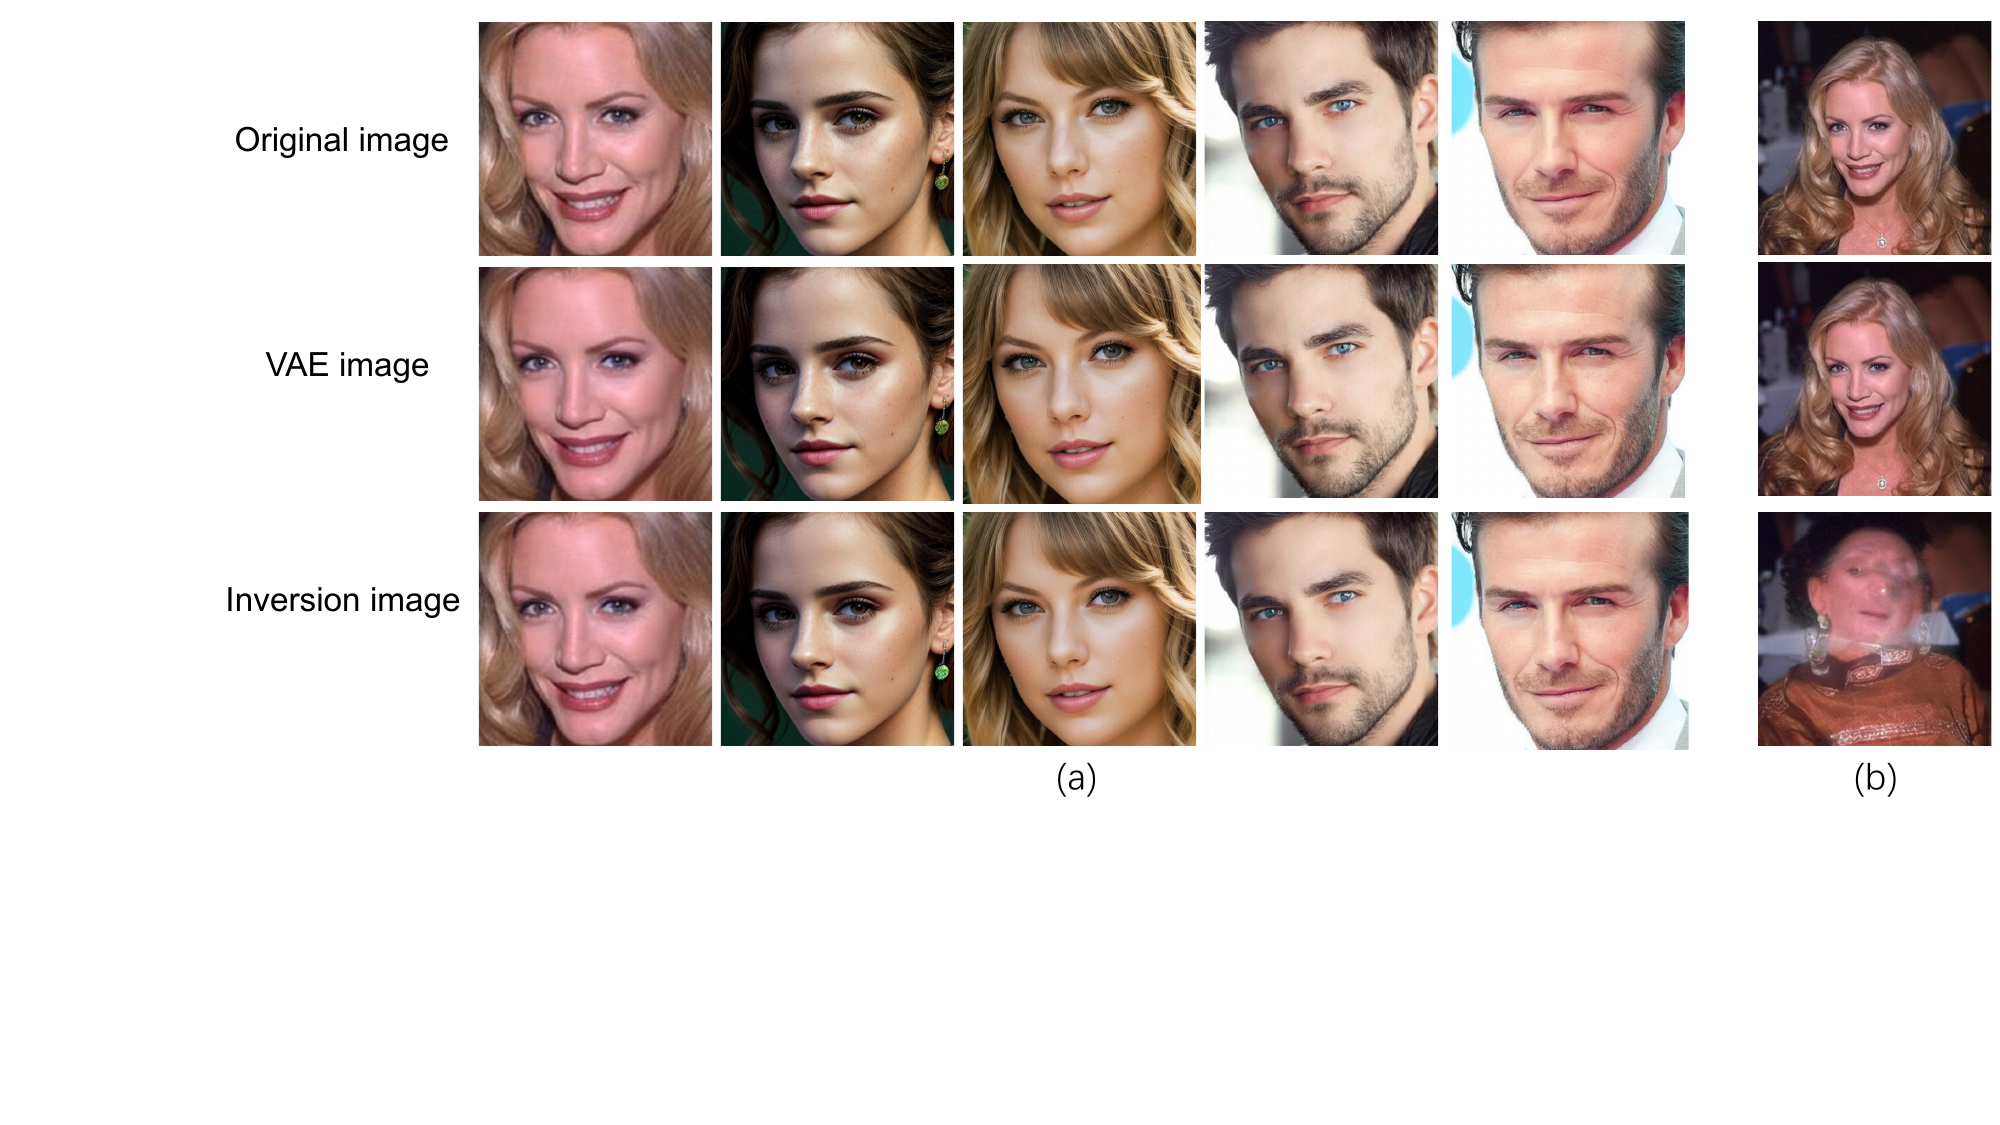}
    \caption{(a) Face images are always recovered with high quality after DDIM inversion. (b) Non-face images lost a lot of information after DDIM inversion. ``Original image'' denotes the input image, ``VAE image'' denotes the image extracted by VAE and then passed through the decoder, and ``Inversion image'' denotes the result of DDIM inversion.}
    \label{fig7}
    \vspace{-0.1cm}
\end{figure}

\begin{figure}[h!]
    \centering\setlength{\abovecaptionskip}{0.1cm}
    \includegraphics[width=0.99\linewidth]{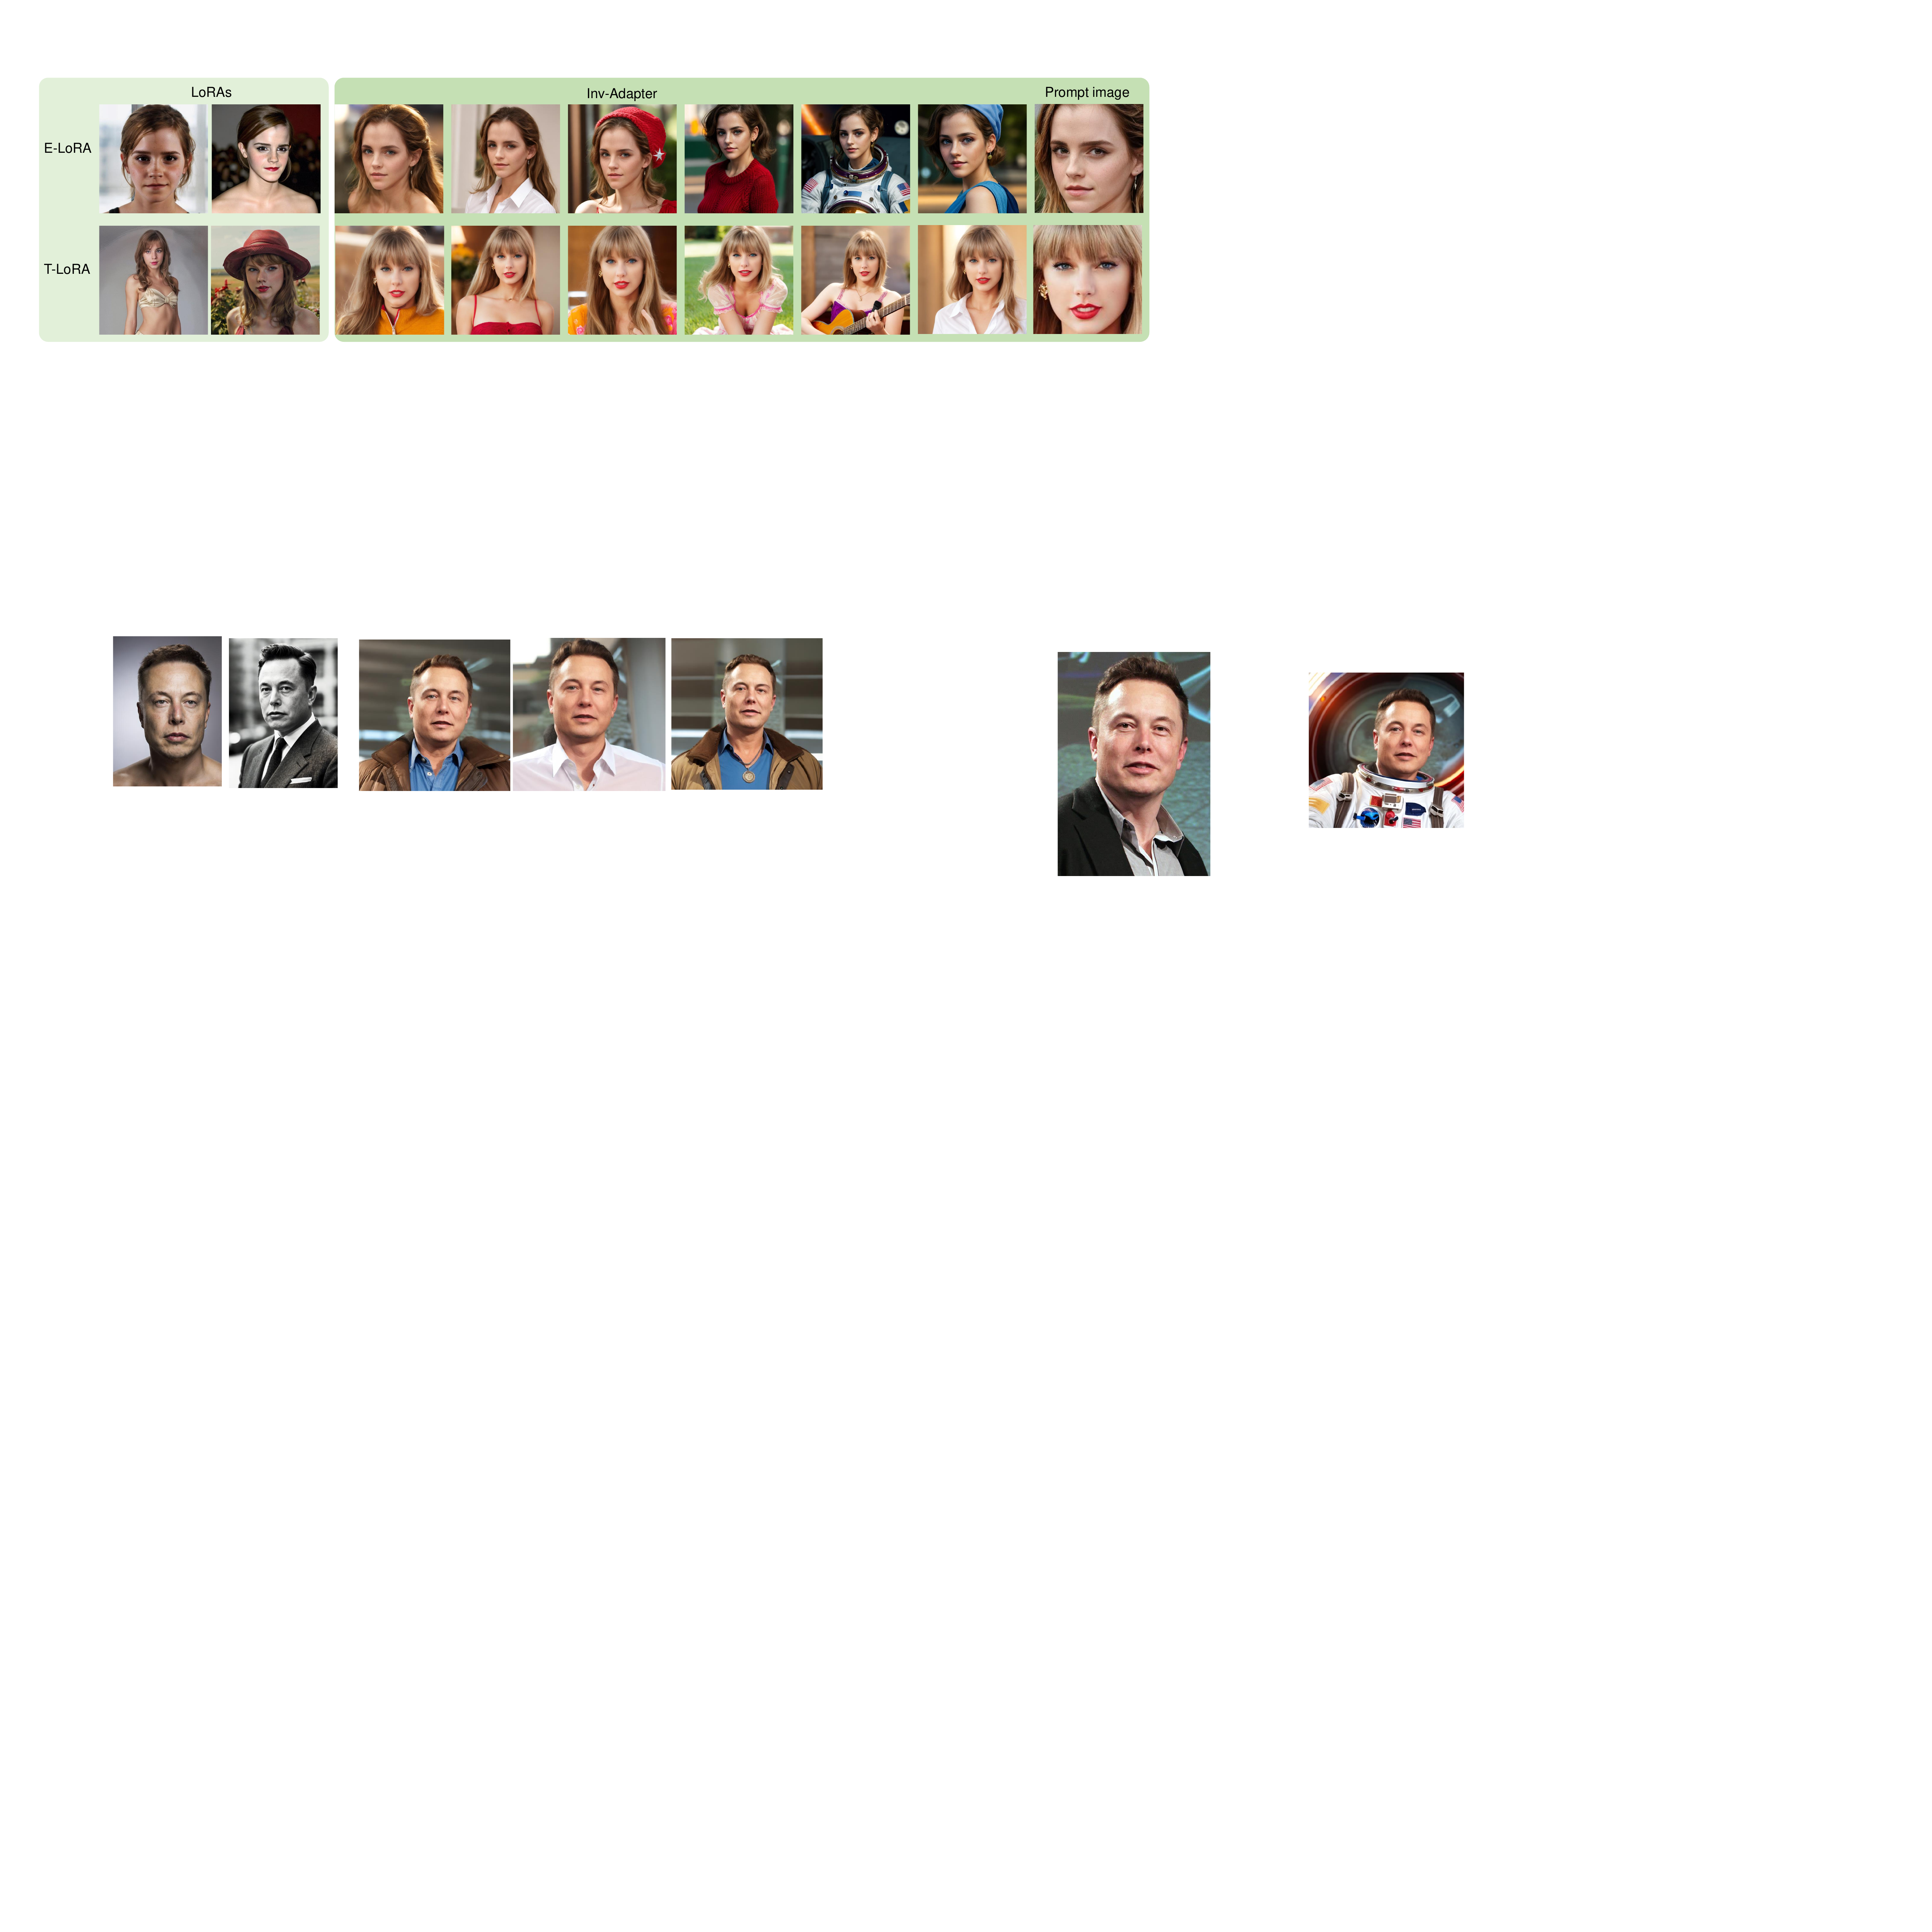}
    \caption{Generation results of the proposed method and LoRAs pre-trained by multiple celebrity images from Civitai. E-LoRA and T-LoRA denote the LoRA trained by Emma Watson and Taylor Swift, respectively.}
    \label{fig7}
    \vspace{-0.1cm}
\end{figure}
\myparagraph{Comparsion with LoRAs.}
To further demonstrate the superiority of Inv-Adapter, we compare the generation results of Inv-Adapter with LoRA models trained on multiple images. 
To this end, we select LoRA models pre-trained using multiple celebrity images, such as Emma Watson\footnote{\scriptsize{\url{https://civitai.com/models/14996?modelVersionId=17669
}}} and Taylor Swift\footnote{\scriptsize{\url{https://civitai.com/models/86858/taylor-swift
}}} from Civitai. 
In Figure~\ref{fig7}, we show the generation results for multiple prompts.
The experimental results mark the competitiveness of our proposed Inv-Adapter, even with specially trained LoRAs.
It is worth mentioning that our approach requires only one image for inference instead of multiple images to fine-tune the text-to-image model, which is more convenient.

\myparagraph{Quantitative Ablation Results for EAA.}
Tables~\ref{tab1} and~\ref{tab2} show the results of the embedded attention adapter (EAA) in the self attention layer only, in the cross attention layer only, and in both self and cross attention layers. 
% %%%%%%%%%%%%%
It can be found that EAA can enhance the generated loyalty only at the self-attention layer, while the ID fidelity is insufficient. 
Meanwhile, both ID fidelity and loyalty of generation can be guaranteed in both cross attention and self attention layers.
\begin{table*}[h]
\setlength{\abovecaptionskip}{0cm}
\setlength{\belowcaptionskip}{-0.01cm}
\centering
\scriptsize
\caption{Ablation results for EAA embeds in self attention layers, cross attention layers, and both layers on the Sample-1k dataset.}
\begin{tabularx}{0.99\textwidth}{>{\centering\arraybackslash}X|>{\centering\arraybackslash}X|>{\centering\arraybackslash}X>{\centering\arraybackslash}X|>{\centering\arraybackslash}X>{\centering\arraybackslash}Xc|>{\centering\arraybackslash}X>{\centering\arraybackslash}X}
\hline
\multirow{2}{*}{Self} &\multirow{2}{*}{Cross} & {BLIP} & {CLIP-T} & {CLIP-I}& {DINO}& {FACE-SIM} & {CLIPIQA} & {FID}  \\
                 &  &                                                                     ($\uparrow$)                     &      ($\uparrow$)                   &       ($\uparrow$)                  &     ($\uparrow$)                  &         ($\uparrow$)                  &     ($\uparrow$)                    &      ($\downarrow$)                             \\ \hline
 \ding{52} &\ding{55} &\textbf{80.78}                &\textbf{ 29.74 }                  & 65.7                   & 55.15                 & 36.70                     & \textbf{88.38 }                   & 240.91               \\
\ding{55}& \ding{52}  & 79.41                 & 28.78                   & 68.85                   & 50.24                 & 55.58                     & 85.00           & 236.24                \\
 \ding{52} &      \ding{52}     & \textbf{}79.65        & 28.45          & \textbf{71.81}          & \textbf{64.33}        & \textbf{65.12}            & 86.80                    & \textbf{228.10}  \\    \hline
\end{tabularx}\label{tab1}
\vspace{-0.7cm}
\end{table*}

\begin{table*}[h]
\setlength{\abovecaptionskip}{0cm}
\setlength{\belowcaptionskip}{-0.01cm}
\centering
\scriptsize
\caption{Ablation results for EAA embeds in self attention layers, cross attention layers, and both layers on the Celebrity dataset.}
\begin{tabularx}{0.99\textwidth}{>{\centering\arraybackslash}X|>{\centering\arraybackslash}X|>{\centering\arraybackslash}X>{\centering\arraybackslash}X|>{\centering\arraybackslash}X>{\centering\arraybackslash}Xc|>{\centering\arraybackslash}X>{\centering\arraybackslash}X}
\hline
\multirow{2}{*}{Self} &\multirow{2}{*}{Cross} & {BLIP} & {CLIP-T} & {CLIP-I}& {DINO}& {FACE-SIM} & {CLIPIQA} & {FID}  \\
                 &  &                                                                     ($\uparrow$)                     &      ($\uparrow$)                   &       ($\uparrow$)                  &     ($\uparrow$)                  &         ($\uparrow$)                  &     ($\uparrow$)                    &      ($\downarrow$)                             \\ \hline
 \ding{52} &\ding{55} &\textbf{83.25}                &\textbf{ 30.47 }                  & 63.23                   & 55.86                 & 35.86                     & \textbf{91.1 }                   & 230.15               \\
\ding{55}& \ding{52}  & 81.73                 & 29.22                   & 70.87                   & 59.85                 & 58.91                     & 88.94           & 220.53                \\
 \ding{52} &      \ding{52}     & 80.04             & {28.21}               & {\textbf{76.79}}               & {\textbf{61.49}}             & \textbf{65.42 }             &\textbf{{89.56} }                        & 201.38    \\    \hline
\end{tabularx}\label{tab2}
\vspace{-0.1cm}
\end{table*}

\myparagraph{Quantitative Ablation Results for Token Aggregation.}
Table~\ref{tab3} shows the results of the quantitative ablation experiments of token aggregation on the two datasets. It is clearly observed that token aggregation can improve ID fidelity. 
% Tables~\ref{tab4} and~\ref{tab5} show the quantitative ablation results of aggregation number on the Sample-1K and Celebrity datasets. The loyalty and ID fidelity tradeoffs are optimal when the aggregation number is 256 or 512.
\begin{table*}[h]
\setlength{\abovecaptionskip}{0cm}
\setlength{\belowcaptionskip}{-0.01cm}
\centering
\scriptsize
\caption{Ablation results for token Aggregation on the Sample-1K and Celebrity datasets.}
\begin{tabularx}{0.99\textwidth}{cc|>{\centering\arraybackslash}X>{\centering\arraybackslash}X|>{\centering\arraybackslash}X>{\centering\arraybackslash}Xc|>{\centering\arraybackslash}X>{\centering\arraybackslash}X}
\hline
Token&\multirow{2}{*}{Dataset}  & {BLIP} & {CLIP-T} & {CLIP-I}& {DINO}& {FACE-SIM} & {CLIPIQA} & {FID}  \\
                  Aggregation&  &                                                                     ($\uparrow$)                     &      ($\uparrow$)                   &       ($\uparrow$)                  &     ($\uparrow$)                  &         ($\uparrow$)                  &     ($\uparrow$)                    &      ($\downarrow$)                             \\ \hline
\multirow{2}{*}{\ding{55}} & Sample-1K & 79.02 & 28.36 & 72.04 & 54.63 & 55.21 & 84.26 & 232.37 \\
                                      &Celebrity      & 78.78 & 28.01 & 75.87 & 58.02 & 58.63 & 87.67 & 238.85 \\ \hline
\multirow{2}{*}{\ding{52}}                    & Sample-1K & 79.65        & 28.45          &71.81         & 64.33        & 65.12            & 86.80                    & 228.10   \\
                                      &Celebrity      & 80.04             & {28.21}               & 76.79             & 61.49            & 65.42            &89.56                       & 201.38 \\ \hline
\end{tabularx}\label{tab3}
\vspace{-0.1cm}
\end{table*}

\begin{wrapfigure}{r}{0.5\textwidth}
    \centering
    \includegraphics[width=.99\linewidth]{pictures/supp2.pdf}
    \caption{Generated results with three different types of diffusion features.}
    \label{figs1}
\end{wrapfigure}
\myparagraph{Ablation Study on Diffusion Features.}
The proposed Inv-Adapter employs different denoising steps to extract different diffusion features. Specifically, we adopt the diffusion feature extracted by $Z_t^p$ after the denoising process at the t-th step. We compare the performance of diffusion features using fixed steps, such as the diffusion features of the 50-th step denoising process (timestep=0) and the intermediate denoising process (timestep=25). The experimental results are shown in Table~\ref{tab6}. 
It can be noticed that the image quality and loyalty are severely degraded as the diffusion features are fixed. Although metrics such as DINO are superior to Inv-Adapter, the generated images are more like direct splices of faces.
We also show the generation results using the three types of methods in Figure~\ref{figs1}. Combining the quantitative results, it can be found that utilizing the diffusion features of each step is more effective.

\begin{table*}[h]
\setlength{\abovecaptionskip}{0cm}
\setlength{\belowcaptionskip}{-0.01cm}
\centering
\scriptsize
\caption{Ablation results for diffusion features on the Sample-1K. ``Fixed'' refers to the use of fixed diffusion features from the denoising process at step $t$. ``Adaptive'' refers to the extraction of diffusion features from each step to inject into the text-to-image generation model, which is adopted by Inv-Adapter.}
\begin{tabularx}{0.99\textwidth}{>{\centering\arraybackslash}X|>{\centering\arraybackslash}X|>{\centering\arraybackslash}X>{\centering\arraybackslash}X|>{\centering\arraybackslash}X>{\centering\arraybackslash}Xc|>{\centering\arraybackslash}X>{\centering\arraybackslash}X}
\hline
\multirow{2}{*}{} &Fixed or& {BLIP} & {CLIP-T} & {CLIP-I}& {DINO}& {FACE-SIM} & {CLIPIQA} & {FID}  \\
              $t $  &                                                              Adaptive&         ($\uparrow$)                     &      ($\uparrow$)                   &       ($\uparrow$)                  &     ($\uparrow$)                  &         ($\uparrow$)                  &     ($\uparrow$)                    &      ($\downarrow$)                             \\ \hline
$0$  &Fixed& 77.84 & 27.54 & 76.6 & 64.6 & 60.75 & 78.34  & 228.96 \\
$25$ &Fixed& 78.92 &28.57&70.94&58.35&58.16&85.84&225.60 \\
$0-50$  &Adaptive& 79.65        & 28.45          &71.81         & 64.33        & 65.12            & 86.80  &228.10 \\
 \hline
\end{tabularx}\label{tab6}
\vspace{-0.1cm}
\end{table*}

\myparagraph{Different Base Model.}
Our Inv-Adapter, once trained, can be adapted to different base models of the same structure. As shown in Figure~\ref{figs2}, we show the generation results of Inv-Adapter trained in SD $v1.5$, employing (1) SD $v1.5$, (2) \textit{Realistic Vision V4.0}, and (3)  \textit{Realistic Vision V6.0} base models from \textit{huggingface}.

\myparagraph{More Visualization Results.} 
Figures~\ref{figs3}-\ref{figs11} show more results of face ID generation. Our proposed Inv-Adapter exhibits strong applicability.

\begin{figure}
    \centering
    \includegraphics[width=.99\linewidth]{pictures/supp1.pdf}
    \caption{Generation results of Inv-Adapter adapted to different base models. (1) denotes SD $v1.5$, (2) denotes \textit{Realistic Vision V4.0}, (3) denotes \textit{Realistic Vision V6.0}.}
    \label{figs2}
\end{figure}

\begin{figure}
    \centering
    \includegraphics[width=.99\linewidth]{pictures/supp3.pdf}
    \caption{Customized generated results of the left ID prompt image using the Inv-Adapter.}
    \label{figs3}
\end{figure}

\begin{figure}
    \centering
    \includegraphics[width=.99\linewidth]{pictures/supp4.pdf}
    \caption{Customized generated results of the left ID prompt image using the Inv-Adapter.}
    \label{figs4}
\end{figure}

\begin{figure}
    \centering
    \includegraphics[width=.99\linewidth]{pictures/supp5.pdf}
    \caption{Customized generated results of the left ID prompt image using the Inv-Adapter.}
    \label{figs5}
\end{figure}

\begin{figure}
    \centering
    \includegraphics[width=.99\linewidth]{pictures/supp6.pdf}
    \caption{Customized generated results of the left ID prompt image using the Inv-Adapter.}
    \label{figs6}
\end{figure}

\begin{figure}
    \centering
    \includegraphics[width=.99\linewidth]{pictures/supp7.pdf}
    \caption{Customized generated results of the left ID prompt image using the Inv-Adapter.}
    \label{figs7}
\end{figure}
\begin{figure}
    \centering
    \includegraphics[width=.99\linewidth]{pictures/supp8.pdf}
    \caption{Customized generated results of the left ID prompt image using the Inv-Adapter.}
    \label{figs8}
\end{figure}

\begin{figure}
    \centering
    \includegraphics[width=.99\linewidth]{pictures/supp9.pdf}
    \caption{Customized generated results of the left ID prompt image using the Inv-Adapter.}
    \label{figs9}
\end{figure}

\begin{figure}
    \centering
    \includegraphics[width=.99\linewidth]{pictures/supp10.pdf}
    \caption{Customized generated results of the left ID prompt image using the Inv-Adapter.}
    \label{figs10}
\end{figure}

% \vspace{-6cm}
\begin{figure*}[t!]
    \centering
    \includegraphics[width=.99\linewidth]{pictures/supp11.pdf}
    \caption{Customized generated results of the left ID prompt image using the Inv-Adapter.}
    \label{figs11}
\end{figure*}
